# Supplementary material for: Fair Representation: Guaranteeing Approximate Multiple Group Fairness for Unknown Tasks
Source: arXiv:2109.00545 source file (2022-02-20)
Supplement: Supplementary file 1 [file tab_MPI3D_appendix.tex]

\begin{table}[h]
    \centering
    \caption{The privacy and discriminativness of our approach with increasing $\lambda$ on correlated MPI3D dataset. Shape completely correlates with color ($|a-b|=1$). The result of privacy and discriminativeness is reported in balanced accuracy. $\uparrow$/$\downarrow$ indicates higher/lower value is better.}
    \label{tab:MPI3D_appendix}
    % \vspace{-1ex}
    % \adjustbox{width=1\columnwidth}{
    \begin{tabular}{l c c c c c}
        \toprule
        \multirow{2}{*}{$\lambda$} &
        Privacy ($\downarrow$) & &
        \multicolumn{3}{c}{Discriminativeness ($\uparrow$)} \\
        \cmidrule{2-2} \cmidrule{4-6}
        &  color (\%)  & & shape  (\%) & size  (\%) & bkgd color (\%)\\ 
        \midrule
        10
        & 67.5{\small \textcolor{gray}{$\pm$1.3}} & &
        67.5{\small \textcolor{gray}{$\pm$1.3}} &
        80.5{\small \textcolor{gray}{$\pm$1.5}} & 
        96.4{\small \textcolor{gray}{$\pm$1.3}} \\

        20
        & 66.2{\small \textcolor{gray}{$\pm$1.5}} & &
        66.2{\small \textcolor{gray}{$\pm$1.5}} &
        77.5{\small \textcolor{gray}{$\pm$2.6}} & 
        95.3{\small \textcolor{gray}{$\pm$1.4}} \\

        40
        & 65.5{\small \textcolor{gray}{$\pm$1.5}} & &
        65.5{\small \textcolor{gray}{$\pm$1.5}} &
        75.0{\small \textcolor{gray}{$\pm$2.0}} & 
        93.4{\small \textcolor{gray}{$\pm$1.7}} \\

        80
        & 65.3{\small \textcolor{gray}{$\pm$1.3}} & &
        65.4{\small \textcolor{gray}{$\pm$1.3}} &
        74.3{\small \textcolor{gray}{$\pm$3.4}} & 
        90.8{\small \textcolor{gray}{$\pm$2.2}} \\
        \bottomrule
    \end{tabular}
\end{table}
